# Supplementary material for: Localize, Group, and Select: Boosting Text-VQA by Scene Text Modeling
Source: arXiv:2108.08965 source file (2021-08-20)
Supplement: Supplementary file 1 [file A_appendix.tex]

\section{Workload Distribution}
\label{sec:work_dist}
We split the tasks as following:

\paragraph{Yansen Wang}
\begin{itemize}
    \item OCR system search \& Evaluation
    \item Question grounding model implementation
    \item Synthtext data augmentation
    \item Beam search implementation
    \item Multi-source OCR combination implementation
\end{itemize}
\paragraph{Xiaopeng Lu}
\begin{itemize}
    \item Code base setup
    \item Baseline result reproduction
    \item Question grounding task design \& data preparation
    \item Question grounding joint training implementation 
\end{itemize}
\paragraph{Zhen Fan}
\begin{itemize}
    \item Error analysis \& Case study
    \item OCR data preparation
    \item OCR BERT implementation
    \item OCR line clustering implementation
    \item Abalations
\end{itemize}
\paragraph{Together}
\begin{itemize}
    \item Idea seeking
    \item Paper writing
\end{itemize}

\section{Failed Attempts}
\label{sec:failures}
In this section, we discuss several ideas which we tried but don't work significantly. 

\subsection{Beam Search}
As a generation task using an auto-regressive method to generate answers, it's possible to add a beam search mechanism to choose from top-k results rather than greedily generate the sequence word by word. We implemented it on LOGOS-base with Azure OCR texts, and the accuracy increased from 0.4775 to 0.4778 which is too small compared to other ideas.

After we analyze the improvements obtained by beam search, we claim that there are two main reasons for the insignificant improvement: 1) Beam search works in tasks such as dialog systems, text summarization where the generated texts are relatively long. However, in this task, the answers are often single word or phrases which are quite short. In these situations, the beam search can't benefit to its maximum. 2) Most of the time, we found that the model is very confident on the output, and the scores of some specific tokens are already high. This makes the beam search rather difficult to change the results.

\subsection{SynthText Data Augmentation}
\begin{figure}
\begin{subfigure}[b]{0.23\textwidth}
    \includegraphics[width=\textwidth]{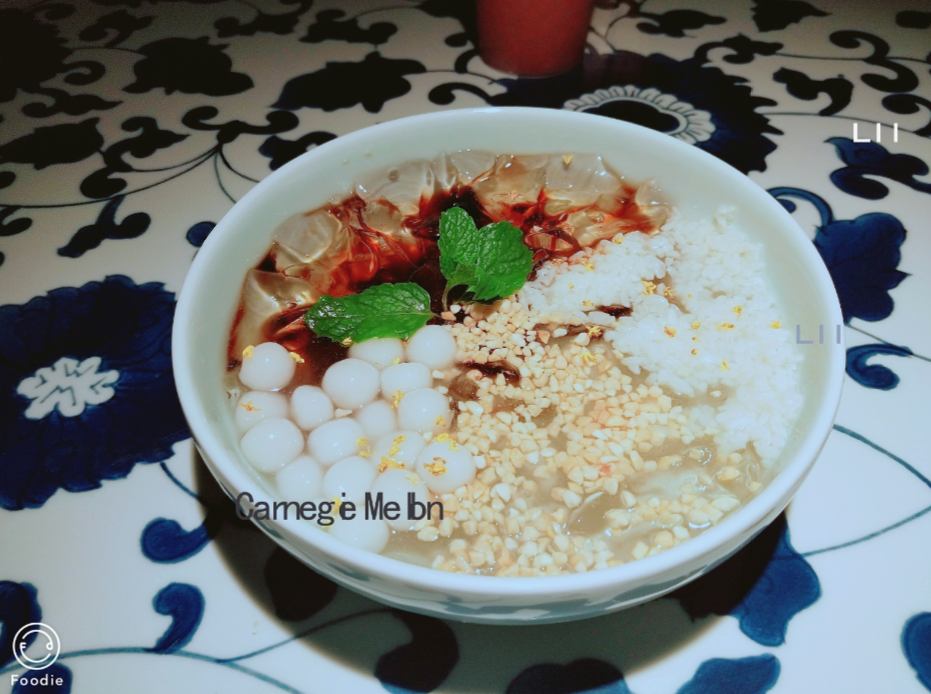}
\end{subfigure}
\hfill
\begin{subfigure}[b]{0.23\textwidth}
    \includegraphics[width=\textwidth]{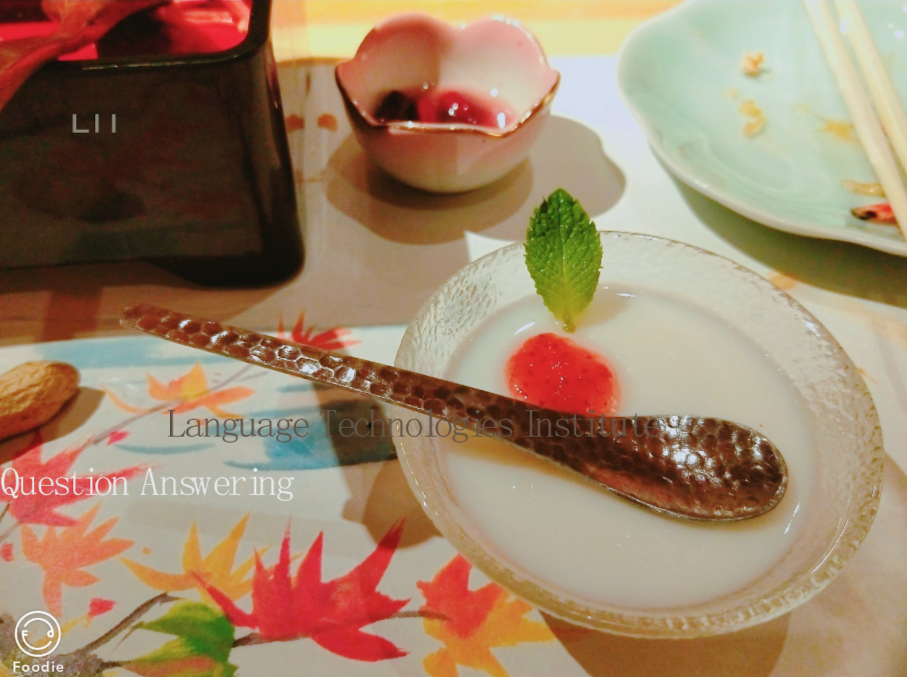}
\end{subfigure}
\caption{Examples of SyntheText generated images}
\end{figure}
Previous research shows that additional OCR training data can boost the model performance~\cite{yang2020tap}. However, doing OCR annotation requires large amounts of computational resources and budget which is beyond our expectation. To alleviate this problem, one way is to generate fake dataset by rendering synthetic text into the image. This method has shown to be effective in OCR research, where OCR training data is not enough. However, when we tried this method, we found that the rendered image is not natural and the text cannot be fully rendered into the image. Therefore, we continued with other idea instead of going forward for SynthText data augmentation idea.

We do think this is a good idea though. Including more diverse OCR training data will likely to improve the results, as the model is likely to be more generalizable given enough training data. In the future, we are planning to continue this idea, and try to generate fake Text-VQA dataset as a data augmentation method.

\iffalse
\fz{List of todos?}
Experiments to run:

- STVQA \\
- LOGOS no grounding \\
- LOGOS no clustering info \\
- LOGOS with only Azure OCR and only Rosetta OCR + clustering \\
- LOGOS with Azure OCR + no grounding, no clustering \\

We need:

- STVQA OCR information \\
- Rosetta clustering \\
\fi
